# Supplementary material for: Aya Vision: Advancing the Frontier of Multilingual Multimodality
Source: arXiv:2505.08751 source file (2025-05-13)
Supplement: Supplementary file 1 [file multimodal_evals_appendix.tex]

\definecolor{highlightcolor}{RGB}{240, 243, 250}
\definecolor{textgray}{gray}{0.5}

\begin{table}[h]
    \small
    \centering
    
    \begin{tabular}{lccccccc}
        \toprule
        Models / Evaluations & \textbf{MaxM} & \textbf{xMMMU} & \textbf{CVQA} & \textbf{MTVQA} & \textbf{Kaleidoscope} & \textbf{xChat} & \textbf{Avg} \\
        \midrule
        Pangea-7B & 53.56 & 44.00 &  \underline{57.20} & 17.97 & 31.31 & 32.21 & 39.38 \\
        Molmo-7B-D & 45.53 & 37.87 & 48.96 &  16.70 & 34.54 & 23.36 & 34.52 \\
        Llama-3.2-Vision-11B & 39.71 & \underline{42.73} & 52.78 & 16.45 & 34.81 & 28.59 & 35.85 \\
        Pixtral-12B  & 46.08 & 42.27 &  52.59 & \underline{19.20} & 33.04  & \textbf{64.50} & \underline{42.95} \\ 
        Qwen-2.5-VL-7B & \textbf{54.72}  & \textbf{46.77} & \textbf{61.69}  & \textbf{28.78}  &  \textbf{39.56} & 58.14  & \textbf{48.28}\\
        \rowcolor{highlightcolor} Aya Vision-8B & \underline{54.64} & 39.94 & 51.32 &  18.05 &   \underline{35.09} & \underline{58.64} & \underline{42.95} \\
        \midrule
        Molmo-72B & \underline{62.37} & 45.41 & 15.88 & 20.60 & 12.56 & 56.09 & 35.49 \\ 
        Llama-3.2-Vision-90B & \textbf{64.81} & \underline{52.40} & \textbf{76.24}  & 
        \underline{27.28} & \underline{45.16} & 51.12 & \underline{52.84} \\
        Qwen-2.5-VL-72B & 58.96 & \textbf{61.74} & \underline{73.71} & \textbf{31.40}  & \textbf{52.94} & \textbf{71.13} & \textbf{58.31} \\
        \rowcolor{highlightcolor} Aya Vision-32B & 59.57 & 45.11 &  62.80 & 22.12 & 38.30 & \underline{70.07} & 49.66 \\
        \bottomrule
    \end{tabular}
    \caption{\textbf{Evaluation on multilingual multimodal academic benchmarks for Aya Vision-8B and Aya Vision-32B together with the baselines}.}
    \label{tab:mm-academic-evals-appendix}
\end{table}
