# Supplementary material for: Aya Vision: Advancing the Frontier of Multilingual Multimodality
Source: arXiv:2505.08751 source file (2025-05-13)
Supplement: Supplementary file 2 [file text_evals_appendix.tex]

\definecolor{highlightcolor}{RGB}{240, 243, 250}
\definecolor{textgray}{gray}{0.5}

\begin{table}[h]
    \small
    \centering
    
    \begin{tabular}{lccccc}
        \toprule
        Models / Evaluations & \textbf{G‑MMLU (Lite)} & \textbf{MGSM} & \textbf{FLORES} & \textbf{IFEval} & \textbf{Avg} \\
        \midrule
        Pangea‑7B             & 46.13      & 50.51      & 28.04       & 23.99  & 37.17   \\
        Molmo‑7B‑D            & 36.97 & 34.78  & 15.74  & 56.10  & 35.90\\
        Llama‑3.2‑11B         & 53.62  & \underline{59.68}  & \underline{31.84}  & \textbf{83.43} & \textbf{57.14} \\
        Pixtral‑12B           & \textbf{61.52}  & \textbf{65.94} & 29.29  & 65.59  & 55.59 \\
        Qwen‑2.5‑VL‑7B        & \underline{59.64}  & 48.27  & 27.98  & 72.46 & 52.09 \\
        \rowcolor{highlightcolor} Aya Vision‑8B   & 56.62  & 50.83  & \textbf{35.90}  & \underline{82.78} & \underline{56.53}  \\
        \midrule
        Molmo‑72B             & 61.71  & \underline{73.53}  & 29.43  & 64.23 & 57.23  \\
        Llama‑3.2‑Vision‑90B  & \underline{72.58}  & 60.72  & \textbf{38.25}  & \underline{88.14} & \underline{64.92}  \\
        Qwen‑2.5‑VL‑72B       & \textbf{76.23}  & \textbf{77.98}  & 35.71  & \textbf{89.74} & \textbf{69.92} \\
        \rowcolor{highlightcolor} Aya Vision‑32B  & 58.46  & 57.61  & \underline{37.79}  & 78.50  & 58.09\\
        \bottomrule
    \end{tabular}
    \caption{Academic Benchmark Results for Aya Vision-8B and Aya Vision-32B. 
    }
    \label{tab:text-only-academic-evals-appendix}
\end{table}
